# Supplementary material for: Generalizing Homophily to Simplicial Complexes
Source: arXiv:2207.11335 source file (2022-07-22)
Supplement: Supplementary file 1 [file data.tex]

The data used in this work falls broadly into six categories depending on the meaning of the interactions.

\begin{itemize}
    \item \texttt{cont} indicates relationships are due to physical contact interactions based on bluetooth proximity.
    Contacts are measured in 20 second intervals, creating a graph of contacts each 20 second period, from which we create simplices from maximal cliques of this graph.
    Node labels are determined by membership in a classroom (\texttt{cont-primary-school}, \texttt{cont-high-school}), specific occupation within a hospital (\texttt{cont-hospital}), household in a village (\texttt{cont-village}), or department within a workplace (\texttt{cont-workplace-13}, \texttt{cont-workplace-15}) \cite{genois2018can,ozella2021using}.
    \item \texttt{bills} details connections via cosponsorship in the United States federal government.
    Simplices form when members of congress cosponsor bills with one another, and nodes are labeled by party affiliation (\texttt{bills-house}, \texttt{bills-senate}) \cite{fowler2006connecting,fowler2006legislative}.
    \item \texttt{email} corresponds to social connections created via email. Simplices form when Enron employees send emails to groups of others, and labels are based on gender of associated nodes (\texttt{email-Enron}) \cite{benson2018simplicial}.
    \item \texttt{hosp} refers to connections due to multiple drugs being used by the same patient in an emergency room.
    Nodes are drugs, and simplices form when an individual enters the emergency room having used multiple drugs. 
    Drugs are labeled based on drug classifications from the Drug Abuse Warning Network (\texttt{hosp-DAWN}) \cite{benson2018simplicial}.
    \item \texttt{soc} refers to social relationships in the context of an online social network.
    Nodes are individuals, and edges represent interactions within the context of the network. 
    Each node is also able to be a member of any number of groups in the social network. 
    $2$-simplices form when three nodes all share edges with one another and there is some group that connects the three nodes.
    The label of a node is given by the group label for which the node has the most mutual edges which are also in that group.
    For these datasets, due to data size restrictions we split the datasets into subsets of roughly 20,000 nodes.
    To ensure sufficiently many $2$-simplices in each subset of 5,000 nodes, we restrict the data to only use nodes that are in the the 10 largest groups for \texttt{soc-youtube}, \texttt{soc-flickr}, and \texttt{soc-livejorunal}, and \texttt{soc-orkut}. \cite{mislove2007measurement}.
    \item \texttt{retail} refers to relationships between hotels in a retail dataset.
    Simplices form when multiple hotels which are browsed during the same user session on the website Trivago.
    Node labels correspond to the country where the hotel is located \cite{benson2018simplicial}.
\end{itemize}
