# Supplementary material for: Generalizing Homophily to Simplicial Complexes
Source: arXiv:2207.11335 source file (2022-07-22)
Supplement: Supplementary file 2 [file experiments.tex]

\subsection{Error Bars in Class-Based Homophily Scores}
\label{aa:error}
To compute error bars in Figure \ref{fig:classbased_comp}, we utilize a standard bootsrapping procedure in which we take random subsets of nodes from the data and compute the class-based homophily scores to compute a standard deviation of the class-based homophily score over 50 trials.
Such error bars are also computed for the global homophily scores in Figure \ref{fig:global_comp} but are negligible.

\subsection{Explained Variance of Homophily Scores}
\label{aa:regs}
To understand the extent to which graph homophily explains hypergraph and $k$-simplicial homophily, we compute the graph homophily score for each dataset as well as both the hypergraph homophily score and the $k$-simplicial homophily score on triangles as described in Section \ref{s:defs}.
Because the scores are distributed exponentially (as can be seen in Figure \ref{fig:global_comp}), we then take logarithm of each score.
We then fit a linear regression model with graph homophily scores as the independent variable, with an offset, and either $k$-simplicial homophily or hypergraph homophily scores as the dependent variable.
We report the $r^2$ score for each linear model, as well as the $p$-value of the coefficient on the graph homophily score.
